# Supplementary material for: Logical Characterization of Coherent Uninterpreted Programs
Source: arXiv:2107.12902 source file (2021-07-26)
Supplement: Supplementary file 1 [file basis_appendix.tex]

\section{Computing $V$-basis}
\hg{TODO: fix alignment, change $rep$}
We describe a procedure that, give a set of EUF literals $\Gamma$ and a set of
constants $V$, computes the $V$-basis abstraction of $\Gamma$: $\base(\Gamma, V)
= \langle W, \beta, \delta \rangle$. The procedure first computes the congruence
closed graph $G$ of $\Gamma$. $G$ is a set of labelled nodes. Each node denotes
a term in $\Gamma^*$. There are directed edges from nodes representing function
applications to each of the function arguments. If $\Gamma^* \vdash t_1 \eq t_2$
then there is an equality edge between nodes of $t_1$ and $t_2$. If $t_1\deq t_2
\in \Gamma$, there is a disequlity edge between $t_1$ and $t_2$. A node
corresponding to term $t$ is labelled using the representative, $rep(t)$, of the
equivalence class $t$ belongs to. Representatives are in the set $V \cup W$: If
$\Gamma^* \vdash v \eq t$ where $v \in V$, then $rep(t) = v$~(we use a fixed
ordering on constants in $V$ to break ties), otherwise $rep(t) = w$ for some $w
\in W$. In this graph,
\begin{multline*}
    \beta = \{ v \eq u \in \Gamma^* \mid v,u \in V\} \cup \hphantom{a} \\
    \{v \deq u \mid v = rep(t_1), u = rep(t_2), t_1 \deq t_2 \in \Gamma, v, u \in V\} \cup \hphantom{a}\\
    \{ v \eq f(rep(t_1), \ldots, rep(t_n)) \mid v \eq f(t_1, \ldots, t_n) \in \Gamma^*, v \in V \}
\end{multline*}
\begin{multline*}
    \delta = \{w \eq u \in \Gamma^* \mid  u \text{ is a constant } \not \in V, w \in W \} \cup \hphantom{a}\\
                \{w \deq u \mid w = rep(t_1), u = rep(t_2), t_1 \deq t_2 \in \Gamma,\\
                \hfill w \in V, u \in V \cup W\} \cup \hphantom{a}\\
            \{ w \eq f(rep(t_1), \ldots, rep(t_n)) \mid w \eq f(t_1, \ldots, t_n) \in \Gamma^* \}
\end{multline*}
